# Supplementary material for: Median bias reduction in random-effects meta-analysis and meta-regression
Source: arXiv:1801.09002 source file (2018-05-23)
Supplement: Supplementary file 1 [file Suppl_KKS.pdf]

# Supplementary material for Median bias reduction in random-effects meta-analysis and meta-regression

Sophia Kyriakou
Department of Statistical Science
University College London
London, WC1E 6BT, UK
sophia.kyriakou.14@ucl.ac.uk

Ioannis Kosmidis
Department of Statistics
University of Warwick
Coventry, CV4 7AL, UK
The Alan Turing Institute
96 Euston Road, London NW1 2DB, UK
Ioannis.Kosmidis@warwick.ac.uk

Nicola Sartori
Department of Statistical Sciences
University of Padova
Via Cesare Battisti, 35121 Padova, Italy
sartori@stat.unipd.it

March 22, 2018

## 1 Introduction

The current report reproduces the statistical analysis of the cocoa intake and the meat consumption data sets as well as the results of the simulation study on meta-analysis as described in the paper "Median bias reduction in random-effects meta-analysis and meta-regression" by S. Kyriakou, I. Kosmidis and N. Sartori. The outputs in the current report have been produced using `R` version 3.4.0 (R Development Core Team, 2017), and the `R` package `metaLik` version 0.42.0 (Guolo and Varin, 2012). The forest plots in Figures 1 and 10 are obtained using the `R` package `metafor` version 2.0.0 (Viechtbauer, 2010).

The file `functionsMMPL.R` provides the following main functions:

- `BiasFit`, which calculates the ML, the maximum mean BRPL, and the maximum median BRPL estimates using the 2-step iterative process described in Section 4.2 of the main paper. The function also returns the standard errors of the fixed-effect parameters.
- `perform_tests`, which calculates the $p$-values and statistics for a single parameter and various alternatives, based on the Wald, the LR, the mean BRPL ratio, and the median BRPL ratio tests.

First we load the required packages and the functions in `functionsMMPL.R`:

```
> library(metaLik)
> library(metatest)
> library(parallel)
> source("functionsMMPL.R")
```

## 2 Analysis of the cocoa intake data

The data for the analysis of the cocoa intake data is

```
> taubert <- data.frame(
+ y = c(-1.90, 1.00, -3.50, -5.90, -4.00),
+ sigma2 = c(0.3442576, 0.8433986, 1.3770304, 1.3770304, 0.2869898),
+ author = c("Study 1","Study 2","Study 3","Study 4","Study 5"))
```

The variable `y` is the diastolic blood pressure change after two weeks of cocoa consumption, and `sigma2` is the variance of the diastolic blood pressure change. The `author` includes the labels of the studies used in the forest plot of the data.

The code chunk below fits the random-effects meta-analysis model with response `y` and summary variances `sigma2`. The model includes an intercept parameter $\beta$ and the heterogeneity parameter $\psi$. The model parameters are estimated using ML, mean BRPL, and median BRPL.

```
> m1 <- metaLik(y ~ 1, data = taubert, sigma2 = sigma2)
> estim <- BiasFit(m1)
> estimates1 <- with(estim, data.frame(ML, MPL, MMPL))
> colnames(estimates1) <- c("ML", "mean BRPL", "median BRPL")
> rownames(estimates1)[2] <- "psi"
> estimates1

                   ML mean BRPL median BRPL
(Intercept) -2.797480 -2.809146   -2.817197
psi          4.217601  5.564933    6.915229
```

The following code chunk calculates the p-value for testing the null hypothesis $\beta = 0$ against the alternative $\beta \neq 0$ using the LR, the mean BRPL ratio and the median BRPL ratio statistics.

```
> pvals <- perform_tests(m1$y, m1$X, m1$sigma2, null = 0,
+                        what = 1, silent = FALSE)[2:4, "pvalues_d"]
> names(pvals) <- c("LR", "mean BRPL ratio", "median BRPL ratio")
> round(pvals,3)

               LR   mean BRPL ratio median BRPL ratio
            0.030             0.053             0.077
```

The chunk of code below simulates 10 000 independent samples of the 5 diastolic blood pressure changes after two weeks of cocoa intake under the ML fit `m1`, conditionally on `sigma2`. For each simulated sample we calculate the ML, maximum mean BRPL, and maximum median BRPL estimators of $\theta = (\beta, \psi)^{\mathrm{T}}$. In addition, $p$-values are computed for testing the null hypothesis $\beta = 0$ against the alternative $\beta \neq 0$ using the LR, the mean BRPL ratio and the median BRPL ratio statistics.

```
> nsimu <- 10000
> simudata <- simulate(m1, nsim = nsimu, seed = 123)
> cl <- makeCluster(7)
> registerDoParallel(cl)
> cres <- foreach(id=seq.int(nsimu), .combine=cbind, .packages=c("metaLik")) %dopar% {
+         mod <- update(m1, data = within(taubert, y <- simudata[, id]))
+         out <- BiasFit(mod)
+         estimates0   <- with(out, c(ML[1], MPL[1], MMPL[1]))
+         estimatespsi <- with(out, c(ML[2], MPL[2], MMPL[2]))
+         pvalues <- perform_tests(simudata[, id], m1$X, m1$sigma2, null = coef(m1)[1],
+                                  what = 1)[2:4, "pvalues_d"]
+         list(estimates0, estimatespsi, pvalues)
+ }
> stopCluster(cl)
```

We use the simulation results to obtain boxplots for the ML, maximum mean BRPL, and maximum median BRPL estimates of $\theta$ (Figure 3), and to calculate the percentage of underestimation for $\psi$ for the ML, mean BRPL, and median BRPL.

```
> ## Extract coefficient estimates for psi
> ml   <- unlist(lapply(cres[2,], `[[`, 1))
> mpl  <- unlist(lapply(cres[2,], `[[`, 2))
> mmpl <- unlist(lapply(cres[2,], `[[`, 3))
> ## % of underestimation
> pu <- 100*c(mean(ml < m1$mle[2]), mean(mpl < m1$mle[2]), mean(mmpl < m1$mle[2]))
> names(pu) <- c("ML", "mean BRPL", "median BRPL")
> pu
> ##     ML   mean BRPL median BRPL
> ## 70.79       59.12       49.35
```

Also, we use the simulation results to calculate the empirical $p$-value distribution (%) for the tests based on the LR, mean BRPL ratio, and median BRPL ratio statistics.

```
> ## Extract p-values for 2-sided test
> pvald_lr    <- unlist(lapply(cres[3,], `[[`, 1))
> pvald_plr   <- unlist(lapply(cres[3,], `[[`, 2))
> pvald_mplr  <- unlist(lapply(cres[3,], `[[`, 3))
> ## Empirical p-value distribution for the LR, mean BRPL ratio, and median BRPL ratio
> pvals <- rbind(pvald_lr,pvald_plr,pvald_mplr)
> alphas <- c(1,2.5,5,10,25,50,75,90,95,97.5,99)/100
> sizes <- sapply(alphas, function(alpha){
+         apply(pvals,1,function(ps) mean(ps < alpha))
+         })
> colnames(sizes) <- format(alphas * 100, digits = 2)
> rownames(sizes) <- c("LR","Mean BRPL ratio","Median BRPL ratio")
> round(sizes * 100, 1)
>
> ##                     1.0  2.5  5.0 10.0 25.0 50.0 75.0 90.0 95.0 97.5 99.0
> ## LR                  5.8  8.4 11.8 18.2 34.6 57.8 79.2 91.8 96.1 98.0 99.2
> ## Mean BRPL ratio     1.6  3.7  6.7 12.1 28.4 52.8 76.6 90.9 95.5 97.9 99.1
> ## Median BRPL ratio  0.6  1.8  4.1  8.6 23.1 48.5 74.2 89.9 94.9 97.5 99.1
```

# 3 Simulation study

The data in this section are simulated from a random-effects meta-analysis model, where the within-study variances are generated from `generate.sigma2s`, where $K$ is the sample size.

```
> generate.sigma2s <- function(K){
+         sigma2s <- 0.25 * rchisq(K, df = 1)
+         ok <- (sigma2s > 0.009 & sigma2s < 0.6)
+         while(sum(ok) < K){
+                 tmp <- 0.25 * rchisq(K-sum(ok), df = 1)
+                 sigma2s[!ok] <- tmp
+                 ok <- (sigma2s > 0.009 & sigma2s < 0.6)
+         }
+         sigma2s
+ }
```

The simulated data are generated from `simulate.BG` conditionally on `sigma2s` and with true parameter values `beta` and `psi`.

```
> simulate.BG <- function(beta,psi,sigma2s) {
+         K <- length(sigma2s)
+         list(y = beta + rnorm(K)*sqrt(psi + sigma2s),
+            y.se = sqrt(sigma2s))
+ }
```

The following code chunk calculates the ML, maximum mean BRPL, and maximum median BRPL estimates of parameter $\theta = (\beta, \psi)^{\mathrm{T}}$, the standard error of the fixed-effect parameter $\beta$, and the $p$-values for testing the null hypothesis $\beta > 0$, $\beta = 0$, or $\beta < 0$ using the LR, the mean BRPL ratio and the median BRPL ratio statistics. Eleven values of the variance component parameter $\psi$ ranging from 0 to 0.1 are chosen, and the number of studies $K$ ranges from 5 to 200. The true value of the fixed-effect parameter $\beta$ is set to 0.5. For each combination of $\psi$ and $K$ considered, we simulate 10 000 data sets and we set the random seed to a given value, here equal to 123, in order to get reproducible results.

```
> ## Variance components to consider
> truepsis <- seq(0, 0.1, length = 11)
> ## Sample sizes to consider
> Ks <- c(seq(5, 50, by = 5), 100, 200)
> ## Other simulation constants
> truebeta <- 0.5
> ## Simulation size per sample size
> nsimu <- 10000
> ## Simulation and computation of estimates, standard errors, and p-values
> z <- 0
> for (i in seq.int(length(Ks))){
+   for (j in 1:length(truepsis)){
+     z <- z+1
+     K <- Ks[i]
+     psi <- truepsis[j]
+     cat("Calculating results for the case K = ", K, ", psi = ", psi, " ...", "\n")
+     ## Generate sigmas and set X
```

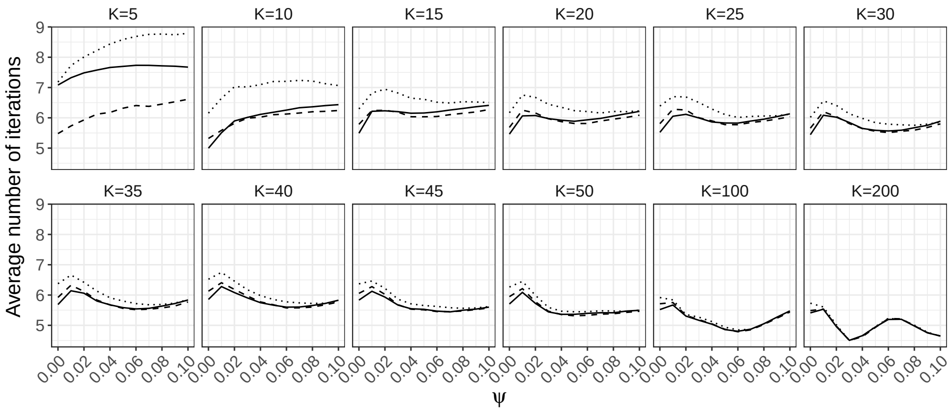


Figure 1: Average number of iterations until the two-step iterative process converges for random-effects meta-analysis for $K \in \{5, 10, 15, 20, 25, 30, 35, 40, 45, 50, 100, 200\}$ and for increasing values of $\psi$ in the interval $[0, 0.1]$. The curves correspond to the maximum median BRPL (solid), maximum mean BRPL (dashed), and ML (dotted) estimators.

```
+     set.seed(123)
+     sigma2 <- generate.sigma2s(K)
+     X <- matrix(1, nrow = K)
+     ## Simulate samples
+     set.seed(123)
+     simuDat <- lapply(seq.int(nsimu), function(k) {
+       dat <- simulate.BG(truebeta,psi,sigma2)
+       data.frame(dat)
+     })
+     ## Get the parameter estimates, the standard errors of beta and the p-values
+     cl <- makeCluster(7)
+     registerDoParallel(cl)
+     cres <- foreach(id=seq.int(nsimu), .combine= cbind, .packages=c("metaLik")) %dopar% {
+       cdat <- simuDat[[id]]
+       m1 <- metaLik(y ~ 1, data = cdat, sigma2 = sigma2)
+       m1BiasFit <- BiasFit(m1)
+       pvalues <- perform_tests(m1$y, m1$X, m1$sigma2, null = truebeta,
+                           what = 1, silent = FALSE)[, c("pvalues_l", "pvalues_d", "pvalues_g")
+       list(estimates = simplify2array(m1BiasFit[1:3]),
+            sterr = simplify2array(m1BiasFit[4:6]),
+            pvalues = pvalues)
+     }
+     stopCluster(cl)
+     save.image(paste0("metanalysis_allK_allpsi", z, ".Rdata"))
+   }
+ }
```

Figures 1 and 2 in the Supplementary material show the average number of iterations and the average computational run-time taken per fit for the two-step iterative process to converge for each value of $K$ and $\psi$ used in the simulation study.

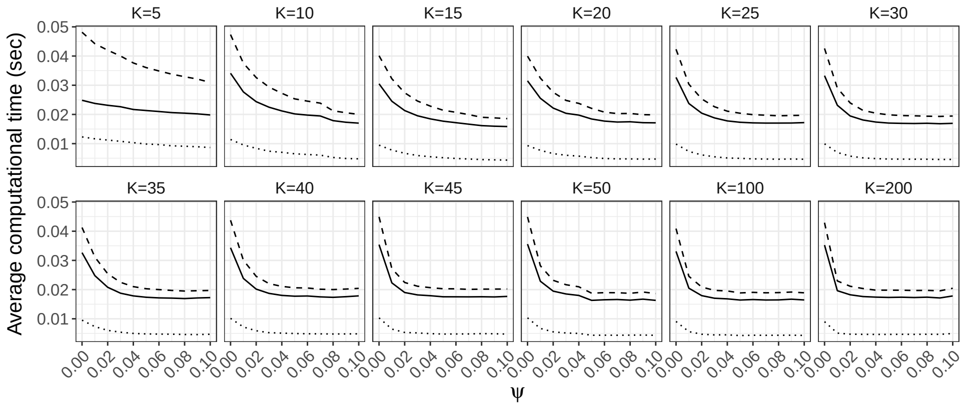


Figure 2: Average computational run-time per fit for random-effects meta-analysis for $K \in \{5, 10, 15, 20, 25, 30, 35, 40, 45, 50, 100, 200\}$ and for increasing values of $\psi$ in the interval $[0, 0.1]$. The curves correspond to the maximum median BRPL (solid), maximum mean BRPL (dashed), and ML (dotted) estimators.

# 4 Analysis of the meat consumption data

The data for the analysis of the meat consumption data is

```
> larsson <- data.frame(
+ y = c(-0.3425, 0.2546, 0.1740, 0.1655,
+           -0.0834, 0.0953, 0.2151, 0.3988,
+           0.0488, 0.1484, 0.2231, 0.2390,
+           0.1823, 0.3577, 0.0583, 0.1484),
+ sigma2 = c(0.017224, 0.001271, 0.000663, 0.005027,
+            0.003383, 0.003603, 0.062186, 0.118504,
+            0.071613, 0.000310, 0.000501, 0.001160,
+            0.000759, 0.005087, 0.031266, 0.023078),
+ type = c(rep("non-p", 8), rep("p", 8)),
+ author = c("Study 1","Study 2","Study 3","Study 4",
+            "Study 5","Study 6","Study 7","Study 8",
+            "Study 9","Study 10","Study 11","Study 12",
+            "Study 13", "Study 14","Study 15","Study 16"))
```

The variable `y` is the logarithm of the relative risk of all-cause mortality for the highest versus the lowest consumption category. The variable `type` represents the meat type (`non-p` for non-processed and `p` for processed) and `sigma2` is the variance of the logarithm of the relative risk. The `author` includes the labels of the studies used in the forest plot of the data.

The code chunk below fits the random-effects meta-regression model with response `y`, explanatory variable `type` and summary variances `sigma2`. The model includes an intercept parameter $\beta_0$, the parameter $\beta_1$ for `type` and the heterogeneity parameter $\psi$. The model parameters are estimated using ML, mean BRPL, and median BRPL.

```
> m1 <- metaLik(y ~ type, data = larsson, sigma2 = sigma2)
> estim <- BiasFit(m1)
> estimates1 <- with(estim, data.frame(ML, MPL, MMPL))
> colnames(estimates1) <- c("ML", "mean BRPL", "median BRPL")
```

```
> rownames(estimates1)[3] <- "psi"
> estimates1

                     ML  mean BRPL median BRPL
(Intercept) 0.099408726 0.09470743  0.09318077
typep       0.106388566 0.10973180  0.11057560
psi         0.008500923 0.01181568  0.01334100
```

The following code chunk calculates the p-value for testing $\beta_1 < 0$ using the LR, the mean BRPL ratio and the median BRPL ratio statistics.

```
> pvals <- perform_tests(m1$y, m1$X, m1$sigma2, null = 0,
+                        what = 2, silent = FALSE)[2:4, "pvalues_g"]
> names(pvals) <- c("LR", "mean BRPL ratio", "median BRPL ratio")
> round(pvals,3)

             LR   mean BRPL ratio median BRPL ratio
          0.047             0.066             0.074
```

The chunk of code below simulates 10 000 independent samples of the 16 logarithms of relative risks under the ML fit `m1`, conditionally on `type` and `sigma2`. For each simulated sample we calculate the ML, maximum mean BRPL, and maximum median BRPL estimators of $\theta = (\beta_0, \beta_1, \psi)^{\mathrm{T}}$. In addition, $p$-values are computed for testing $\beta_1 < 0$ using the LR, the mean BRPL ratio and the median BRPL ratio statistics.

```
> nsimu <- 10000
> simudata <- simulate(m1, nsim = nsimu, seed = 123)
> cl <- makeCluster(7)
> registerDoParallel(cl)
> cres <- foreach(id=seq.int(nsimu), .combine=cbind, .packages=c("metaLik")) %dopar% {
+         mod <- update(m1, data = within(larsson, y <- simudata[, id]))
+         out <- BiasFit(mod)
+         estimates0   <- with(out, c(ML[1], MPL[1], MMPL[1]))
+         estimates1   <- with(out, c(ML[2], MPL[2], MMPL[2]))
+         estimatespsi <- with(out, c(ML[3], MPL[3], MMPL[3]))
+         pvalues <- perform_tests(simudata[, id], m1$X, m1$sigma2, null = coef(m1)[2],
+                                  what = 2)[2:4, "pvalues_g"]
+         list(estimates0, estimates1, estimatespsi, pvalues)
+ }
> stopCluster(cl)
```

We use the simulation results to obtain boxplots for the ML, maximum mean BRPL, and maximum median BRPL estimates of $\theta$ (Figure 11), and to calculate the percentage of underestimation for $\psi$ for the ML, mean BRPL, and median BRPL.

```
> ## Extract coefficient estimates for psi
> ml   <- unlist(lapply(cres[3,], `[[`, 1))
> mpl  <- unlist(lapply(cres[3,], `[[`, 2))
> mmpl <- unlist(lapply(cres[3,], `[[`, 3))
> ## % of underestimation
> pu <- 100*c(mean(ml < m1$mle[3]), mean(mpl < m1$mle[3]), mean(mmpl < m1$mle[3]))
```

```
> names(pu) <- c("ML", "mean BRPL", "median BRPL")
> pu
> ##     ML   mean BRPL median BRPL
> ## 72.56       56.56       49.87
```

Also, we use the simulation results to calculate the empirical $p$-value distribution (%) for the tests based on the LR, mean BRPL ratio, and median BRPL ratio statistics.

```
> ## Extract p-values for 1-sided test
> pvalg_lr    <- unlist(lapply(cres[4,], `[[`, 1))
> pvalg_plr   <- unlist(lapply(cres[4,], `[[`, 2))
> pvalg_mplr  <- unlist(lapply(cres[4,], `[[`, 3))
> ## Empirical p-value distribution for the LR, mean BRPL ratio, and median BRPL ratio
> pvals <- rbind(pvalg_lr,pvalg_plr,pvalg_mplr)
> alphas <- c(1,2.5,5,10,25,50,75,90,95,97.5,99)/100
> sizes <- sapply(alphas, function(alpha){
+        apply(pvals,1,function(ps) mean(ps < alpha))
+        })
> colnames(sizes) <- format(alphas * 100, digits = 2)
> rownames(sizes) <- c("LR","Mean BRPL ratio","Median BRPL ratio")
> round(sizes * 100, 1)
>
> ##                     1.0  2.5  5.0 10.0 25.0 50.0 75.0 90.0 95.0 97.5 99.0
> ## LR                  2.2  4.5  7.7 13.1 28.0 50.0 71.7 86.6 92.1 95.3 97.7
> ## Mean BRPL ratio     1.3  3.0  5.6 11.1 25.9 49.8 73.8 89.0 94.2 96.9 98.6
> ## Median BRPL ratio  1.0  2.5  4.9  9.9 25.1 49.7 74.7 89.8 94.8 97.5 98.9
```

# References


[1] Guolo, A. and Varin, C. (2012). The R package metaLik for likelihood inference in meta-analysis. *J. Stat. Softw.* **50**, 1–14.

[2] R Development Core Team (2017). *R: A Language and Environment for Statistical Computing.* Vienna, Austria: R Foundation for Statistical Computing. http://www.R-project.org.

[3] Viechtbauer, W. (2010). Conducting meta-analyses in R with the metafor package. *J. Stat. Softw.* **36**, 1–48.
